# Supplementary material for: A first-principles machine-learning force field for heterogeneous ice nucleation on microcline feldspar
Source: arXiv:2305.10255 ancillary file (2023-05-17)
Supplement: Supplementary file 1 [file SupplementaryInformation.pdf]

# Electronic Supplementary Information to: A first-principles machine-learning force field for heterogeneous ice nucleation on microcline feldspar

Pablo M. Piaggi,[a] Annabella Selloni,[a] Athanassios Z. Panagiotopoulos ,[b] Roberto Car[a,c], and Pablo G. Debenedetti[b]

## Contents

**1 Electronic structure calculations** 1

**2 Machine-learning model definition and training** 1

**3 Molecular dynamics simulations** 2

**4 Enhanced sampling simulations** 2

**5 Initial training data** 3

**6 Active learning** 4

**7 Calculation of surface energies** 4

**8 Formation of ice cluster at the microcline/water interface** 5

## 1 Electronic structure calculations

Plane-wave DFT calculations were performed using the QUANTUM ESPRESSO suite for electronic structure calculations v6.4.1[1,2] The SCAN exchange and correlation functional[3,4] was evaluated with the LIBXC 4.3.4 library[5] We employed norm-conserving, scalar-relativistic pseudopotentials[6] for K, Al, Si, O, H parametrized using the PBE[7] functional with 9, 11, 4, 6, and 1 valence electrons, respectively. Kinetic energy cutoffs of 110 and 440 Ry were used for the wave functions and the charge density. $k$-point convergence was evaluated for each configuration with energy convergence threshold 1 meV/atom. The convergence absolute error for the self-consistent procedure was set to $10^{-6}$ Ry. For energy minimization with respect to the box or atomic coordinates, the criterion for ending the minimization was a change in energy smaller than $10^{-4}$ Ry in subsequent iterations. For surface configurations, we employed a dipole correction based on a saw-like potential in the direction perpendicular to the interface[8]. The mixing factor for self consistency was set to 0.5. All other parameters were set to their default values in QUANTUM ESPRESSO.

[a] *Department of Chemistry, Princeton University, Princeton, NJ 08544, USA*
[b] *Department of Chemical and Biological Engineering, Princeton University, Princeton, NJ 08544, USA*
[c] *Department of Physics, Princeton University, Princeton, NJ 08544, USA*

## 2 Machine-learning model definition and training

Machine-learning interatomic potentials were constructed using the Deep Potential methodology developed by Zhang *et al.*[9] as implemented in the DEEPMD-KIT v2.0.0.b2[10]. Below, we describe the smooth version of this framework[11], which is based on deep neural networks and descriptors learned on the fly during the training process.

The total energy $E$ of a configuration of $N$ atoms with atomic coordinates $\mathbf{R}$ is written as a sum over per-atom energies $E_i$, i.e,

$$E(\mathbf{R}) = \sum_{i=1}^{N} E_i = \sum_{i=1}^{N} E^{\alpha_i}(\mathbf{R}_i) \tag{1}$$

where $\mathbf{R}_i$ are the relative atomic coordinates of $N_i$ neighbors in an environment with cutoff $r_c$ around atom $i$, $\alpha_i$ is the atom type of atom $i$, and $E^{\alpha_i}$ is an energy function for atoms of the chemical species $\alpha_i$. In order to preserve the natural symmetries of the problem, i.e., rotation and permutation of atoms of the same type, we define a vector of descriptors $\mathbf{D}_i$ for atom $i$. Then, the energy of a configuration can be written as,

$$E(\mathbf{R}) = \sum_{i=1}^{N} E^{\alpha_i}(\mathbf{D}_i). \tag{2}$$

The starting point for the definition of the descriptors $\mathbf{D}_i$ is a continuous and differentiable switching function,

$$s(r) = \begin{cases} \frac{1}{r}, & r < r_s \\ \frac{1}{r}\left\{u^3\left(-6u^2+15u-10\right)+1\right\}, & r_s \leq r < r_c \\ 0, & r \geq r_c \end{cases} \tag{3}$$

where $u = (r - r_s)/(r_c - r_s)$, and $r_s$ and $r_c$ are smooth and hard cutoffs, respectively. Next, we construct a matrix $\tilde{\mathbf{R}}_i \in \mathbb{R}^{N_i \times 4}$ of generalized coordinates with rows,

$$(\tilde{\mathbf{R}}_i)_j = \left[ \begin{array}{cccc} s(r_{ij}), & \frac{s(r_{ij})x_{ij}}{r_{ij}}, & \frac{s(r_{ij})y_{ij}}{r_{ij}}, & \frac{s(r_{ij})z_{ij}}{r_{ij}} \end{array} \right] \tag{4}$$

where $(x_{ij}, y_{ij}, z_{ij})$ is the distance vector from atom $j$ to atom $i$, and $r_{ij}$ is the norm of such distance. Furthermore, we define an embedding matrix $\mathbf{G}^i \in \mathbb{R}^{N_i \times M_1}$ with row $j$ given by,

$$(\mathbf{G}^i)_{j,*} = g^{\alpha_i,\alpha_j}\left(s(r_{ij})\right) \tag{5}$$

where $g^{\alpha_i,\alpha_j}$ is a function that maps a scalar into $M_1$ outputs, and is different for each pair of chemical species $\alpha_i$ and $\alpha_j$. We also define a secondary embedding matrix $\mathbf{G}'^i \in \mathbb{R}^{N_i \times M_2}$ with the first $M_2 < M_1$ columns of $\mathbf{G}^i$. With these ingredients, we now write the descriptor matrix $\mathbf{D}_i \in \mathbb{R}^{M_1 \times M_2}$ as,

$$\mathbf{D}_i = (\mathbf{G}^i)^T \tilde{\mathbf{R}}_i (\tilde{\mathbf{R}}_i)^T \mathbf{G}'^i \tag{6}$$

which is subsequently flatten into a vector of $M_1 \times M_2$ elements and is used as input in Eq. (2). In our simulations, we used a model for five chemical species $\boldsymbol{\alpha}$=(K,Al,Si,O,H), $E^{\alpha_i}$ in Eq. (2) was represented by a neural network with three layers and 120 neurons per layer, and $g^{\alpha_i,\alpha_j}$ in Eq. (5) was represented by a three-layer neural network with sizes 25, 50 and 100, respectively. Other parameters of our model are $M_1 = 100$, $M_2 = 16$, $r_s = 3$ Å, and $r_c = 6$ Å.

The parameters in the neural networks $E^{\alpha_i}$ and $g^{\alpha_i,\alpha_j}$ described above are determined through the minimization of the following loss function,

$$\mathscr{L} = \frac{1}{N_{\mathscr{B}}} \left( \sum_{l \in \mathscr{B}} \frac{w_\varepsilon}{N_l} \left| E_l - E(\mathbf{R}^l) \right|^2 + \frac{w_f}{3N_l} \left\| \mathbf{F}_l - \mathbf{F}(\mathbf{R}^l) \right\|^2 \right) \tag{7}$$

where $\mathscr{B}$ is a mini-batch (i.e., a subset of the training set) with $N_{\mathscr{B}}$ atomic configurations, $w_\varepsilon$ and $w_f$ are weights, $E_l$ and $\mathbf{F}_l$ are reference energies and forces, $E(\mathbf{R}^l)$ and $\mathbf{F}(\mathbf{R}^l) = -\nabla_{\mathbf{R}} E(\mathbf{R}^l)$ are the energy and force predictions of our model described in Eq. (2) for configuration $l$ in the minibatch, and $\mathbf{R}^l$ and $N_l$ are the atomic coordinates and the number of atoms in configuration $l$. The parameters in the training procedure were as follows. We trained the models using the Adam optimizer with learning rate $\alpha(i) = \alpha_0 \lambda^{i/\tau}$ where $\alpha_0 = 0.002$ is the initial learning rate, $\lambda = 0.97$, $\tau = 5 \times 10^3$, and $i$ is the step number. The batch size $N_{\mathscr{B}}$ was set to one and we trained for a total number of steps equal to $2 \times 10^6$. $w_\varepsilon$ and $w_f$ were varied according to $w_\varepsilon(i) = w_\varepsilon^1 + (w_\varepsilon^0 - w_\varepsilon^1)\lambda^{i/\tau}$ and $w_f(i) = w_f^1 + (w_f^0 - w_f^1)\lambda^{i/\tau}$, with $w_\varepsilon^0 = 0.02$, $w_\varepsilon^1 = 1$, $w_f^0 = 1000$, and $w_f^1 = 1$. This scheme gives a higher weight to the force term in Eq. (7) at the beginning of the training process, and by the end of it both the energy and force term have equal weights. After the training process, the model was subsequently compressed as described in ref. 12 in order to improve the computational performance.

An example of the training curves resulting from the protocol described above is shown in Fig. 1.

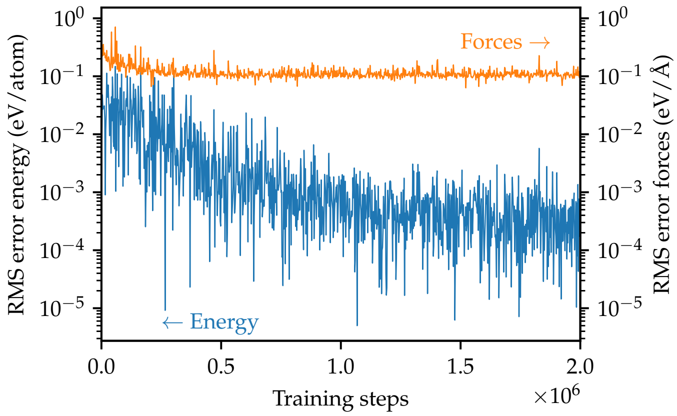


Fig. 1 Training curve for the machine learning model of the potential energy surface of liquid water, ice, microcline feldspar, feldspar/vacuum interfaces, and feldspar/water interfaces. The root mean square (RMS) error in energy and forces is shown as a function of the training steps.

## 3 Molecular dynamics simulations

We performed molecular dynamics simulations using LAMMPS[13,14]. The time step for the integration of the equations of motion was 0.5 fs. We used the standard atomic weights for the masses of all elements (K, Al, Si, O) except H, for which we used a mass of 2 grams/mol, in order to improve the stability of the integration of the equations of motion. We controlled the temperature using the stochastic velocity-rescaling thermostat[15] with a relaxation time of 0.1 ps.

For constant pressure simulations we employed a Parrinello-Rahman barostat with relaxation time 1 ps. For the simulation of bulk liquid water we used an isotropic barostat (box vector lengths coupled, and angles fixed) and for bulk ice $I_h$ we used a fully anisotropic barostat (box vector lengths and angles can vary independently). In both cases we employed systems with 288 water molecules.

## 4 Enhanced sampling simulations

Enhanced sampling simulations were carried out using the enhanced sampling plugin PLUMED[16,17]. We employed the global Steinhardt parameter $Q_6$ as collective variable[18–20], which we define below. We first consider the local Steinhardt parameter for oxygen atom $i$,

$$q_{6m}(i) = \frac{\sum_j \sigma(r_{ij}) Y_{6m}(\mathbf{r}_{ij})}{\sum_j \sigma(r_{ij})} \tag{8}$$

where the sums run over all neighboring oxygen atoms $j$ closer than a distance $r_2$ (defined below), $\mathbf{r}_{ij}$ is the distance vector between $i$ and $j$ with norm $r_{ij} = |\mathbf{r}_{ij}|$, $Y_{6m}$ are spherical harmonic with $l = 6$, and $-6 < m < 6$ is an integer. The switching function $\sigma(r_{ij})$ makes $q_{6m}(i)$ continuous and

differentiable and is defined as,

$$\sigma(r_{ij}) = \begin{cases} 1 \quad \text{if} \quad y < 0 \\ (y-1)^2(1+2y) \quad \text{if} \quad 0 < y < 1 \\ 0 \quad \text{if} \quad y > 1 \end{cases}, \tag{9}$$

with $y = (r_{ij} - r_1)/(r_2 - r_1)$, $r_1 = 0.3$ nm, and $r_2 = 0.35$ nm. The values of $r_1$ and $r_2$ were chosen based on the position of the first peak of the radial distribution function, such that $\sigma(r_{ij}) \approx 1$ for first neighbors and $\sigma(r_{ij}) \approx 0$ for more distant neighbors.

Using $q_{6m}(i)$ described above, we define the global Steinhardt order parameter as,

$$Q_6 = \sqrt{\frac{4\pi}{2l+1} \sum_{m=-l}^{l} \left| \frac{1}{N} \sum_{i=1}^{N} q_{6m}(i) \right|^2} \tag{10}$$

where $l = 6$, and $N$ is the total number of oxygen atoms for which $q_{6m}(i)$ was calculated. This quantity was used to drive the formation of ice in the microcline/water interfacial systems used during the active learning procedure.

In large simulation boxes, biasing $Q_6$ leads to the formation of ice throughout the simulation box, instead of localized in a region of space, as expected in nucleation phenomena. For this reason, we used a variant of $Q_6$, denoted $Q_6^{\text{sph}}$, which localizes the effect of the collective variable in a spherical region centered at a position $\mathbf{r}^0$. We define this collective variable in the following way,

$$Q_6^{\text{sph}} = \sqrt{\frac{4\pi}{2l+1} \sum_{m=-l}^{l} \left| \frac{\sum_{i=1}^{N} \gamma(r_{i0})\, q_{6m}(i)}{\sum_{i=1}^{N} \gamma(r_{i0})} \right|^2} \tag{11}$$

where $r_{i0} = |\mathbf{r}_i - \mathbf{r}^0|$ is the distance from the $i$-th oxygen atom to a reference position $\mathbf{r}^0$ (center of the sphere), which we define as the position of a K atom at the microcline/water surface, and other symbols have the same meaning as above. The switching function $\gamma(r_{i0})$ was defined as,

$$\gamma(r_{i0}) = 1 - \tanh(r_{i0}/r^*) \tag{12}$$

with $r^* = 1.5$ nm, $Q_6^{\text{sph}}$ was used to drive the formation of ice the large microcline/water interfaces described in the main part of manuscript.

## 5 Initial training data

The starting point for training the machine-learning model consisted in configurations of bulk microcline feldspar, bulk water and ice Ih, and feldspar surfaces in contact with liquid water. The procedure to obtain such configuration is described below.

**Microcline feldspar** The initial configuration for microcline feldspar was obtained from the American Mineralogist Crystal Structure Database and corresponds to the experimental structure determined in ref. 21. Experiments show that Al and Si can exhibit disorder in the four non-equivalent sites $T_1(0)$, $T_1(m)$, $T_2(0)$, and $T_2(m)$. The probability of finding Si in each of these sites is in the ranges 0.23-0.52, 0.64-0.87, 0.92-0.98, and 0.92-0.98, respectively[21–23]. We made the simplification of assigning Al to $T_1(0)$ sites, and Si to $T_1(m)$, $T_2(0)$, and $T_2(m)$. Thus, our microcline configurations do not show Al/Si disorder, and the stoichiometry is exactly $KAlSi_3O_8$.

We first minimized the energy of the microcline structure with respect to the cell dimensions and the atomic coordinates using DFT and the SCAN functional. The configuration contained 52 atoms, corresponding to 4 formula units. The lattice constants thus obtained are reported and discussed in the Results section below. Starting from the relaxed configuration, we perturbed randomly the atomic coordinates and box dimensions to generate structures that sample the potential energy surface of bulk feldspar. Each atomic coordinate is displaced by $\delta R = \delta R_{\text{max}}(2x-1)$ where $\delta R_{\text{max}}$ is the maximum displacement and $x \in (0,1)$ is a random number, and each box dimension $L$ is scaled with $L = L_0[1 + \varepsilon^L_{\text{max}}(2x-1)]$ where $L_0$ is the initial box dimension and $\varepsilon^L_{\text{max}}$ is the maximum fractional change in box dimensions. The number of perturbed configurations and the parameters used are summarized in Table 1.

**Bulk water, ice $I_h$, and ice $I_c$** In order to obtain initial configurations for bulk water, ice $I_h$, and ice $I_c$ we used trajectories from our previous work[24–26], which were driven by a previously trained DeePMD model[27]. Information about these simulations and the methodology for extracting frames from the trajectories is given in Table 2. In total, around 1000 configurations of liquid water, ice $I_h$, and ice $I_h$ were used. Note that in two of the simulations liquid water and ice were sampled reversibly[24]. Thus, the training data includes interfacial configurations and ice configurations with diverse proton arrangements (proton disor-

Table 1 Parameters for the generation of microcline feldspar configurations with randomly perturbed atomic coordinates and box dimensions. $\delta R_{\text{max}}$ is the maximum displacement of atomic coordinates and $\varepsilon^L_{\text{max}}$ is the percent change in box dimensions.

| # configurations | $\delta R_{\text{max}}$ (Å) | $\varepsilon^L_{\text{max}}$ (%) |
|---|---|---|
| 100 | 0.01 | 1 |
| 100 | 0.05 | 2 |
| 100 | 0.1 | 3 |
| 10 | 0.2 | 5 |

der). Although most simulations were performed at constant pressure 1 bar, we also employed a simulation at 3200 bar which is below the liquid-liquid critical point[26]. We used these simulation trajectory to provide the model with examples of the atomic environments in the low-density liquid (LDL) and high-density liquid (HDL)[28].

**Feldspar surfaces** We constructed feldspar surfaces with the (100), (010), and (001) crystallographic planes exposed to vacuum. We identified several terminations for each surface and we saturated all undercoordinated oxygen atoms with protons. For each of the studied terminations, we minimized the energy with respect to the atomic coordinates. Then we generated ten perturbed configurations for each of the terminations and the $\delta R_{\max}$-$\varepsilon^L_{\max}$ parameters in Table 1. The surface configurations contained between 58 and 128 atoms.

## 6 Active learning

With the data described above, we trained an initial ensemble of four models, with different initialization random seeds. The models were subsequently improved with an active learning procedure. This approach is iterative and each iteration $k$ can be described as follows,

1. use the models obtained in iteration $k-1$ to run molecular dynamics simulations. The simulations are described in detail below.

2. extract high-error configurations from the resulting trajectories. The error $\varepsilon_i$ in the $i$-th force component is calculated as proposed in ref. 29, i.e, $\varepsilon_i^2 = \langle |f_i - \bar{f}_i|^2 \rangle$, where $\bar{f}_i = \langle f_i \rangle$ and the average $\langle \cdot \rangle$ is taken over the ensemble of models. The errors were evaluated every 0.25 ps and high-error configurations were defined by a maximum error in the forces $\varepsilon = \max_i \varepsilon_i > 0.2$ eV/Å.

3. compute energies and forces of the extracted configurations via DFT calculations (see section on electronic-structure calculations for further details).

4. train a new set of four models which correspond to iteration $k$. The data for the models in iteration $k$ includes all or a subset of the data obtained in iterations $i = 1, ..., k$.

This process was repeated until the convergence criterion $\max_i \varepsilon_i < 0.2$ eV/Å was met. Around 20 iterations were needed to reach the desired accuracy.

In Fig. 1 we show the training curves for the final machine learning model of the *ab initio* potential energy surface obtained in this work.

**Feldspar/water and feldspar/ice interfaces** Configurations for the active learning process were generated using molecular dynamics simulations of the water/feldspar interface at constant volume, and constant temperature equal to 300 K (7 K of supercooling). We used the most stable terminations for the (100), (010), and (001) surfaces of feldspar. The configurations contained 544, 900, and 664 atoms, respectively. Since the water to ice transition is a rare event in the time scale accessible to a molecular simulation, we used advanced sampling to observe this phase transformation at feldspar surfaces during our simulations. This was achieved through a harmonic bias potential,

$$V(Q_6(\mathbf{R})) = \frac{k}{2}\left(Q_6(\mathbf{R}) - Q_6^{\mathrm{ctr}}(t)\right)^2 \tag{13}$$

where $k = 10^5$ kJ/mol, $Q_6(\mathbf{R})$ is the Steinhardt parameter defined above, and $Q_6^{\mathrm{ctr}}(t) = Q_6^0 + (Q_6^f - Q_6^0)t/t_{\mathrm{tot}}$ is the center of the harmonic bias which changes linearly with time $t$ from initial value $Q_6^0$ to final value $Q_6^f$ over the total simulation time $t_{\mathrm{tot}} = 1$ ns. $Q_6^0 \approx 0$ and $Q_6^f = 0.55$ are values of $Q_6(\mathbf{R})$ compatible with liquid water and ice, respectively.

## 7 Calculation of surface energies

We evaluated the zero-temperature stability of different surfaces and terminations as follows. We consider slab configurations with two identical surface terminations which can be described as $N_f$ unit formulas of bulk feldspar plus $N_w$ water molecules,

$$N_f\,\mathrm{KAlSi_3O_8(bulk)} + N_w\,\mathrm{H_2O(g)} \rightarrow \mathrm{K}_{N_f}\mathrm{Al}_{N_f}\mathrm{Si}_{3N_f}\mathrm{O}_{8N_f+N_w}\mathrm{H}_{2N_w}\mathrm{(slab)} \tag{14}$$

The potential energy of the slab configurations can be written as,

$$E_{\mathrm{slab}} = N_f E^{\mathrm{bulk}}_{\mathrm{feldspar}} + N_w E^{\mathrm{gas}}_{H_2O} + 2A\gamma \tag{15}$$

where $E^{\mathrm{bulk}}_{\mathrm{feldspar}}$ is the potential energy of bulk feldspar, $E^{\mathrm{gas}}_{H_2O}$ is the potential energy of an isolated water molecule, $A$ is the surface area, and $\gamma$ is the surface energy. Eq. (15) is only valid in the limit $N_f \rightarrow \infty$, when the slab is infinitely thick. As proposed by Fiorentini and Methfessel[30], we first compute $E_{\mathrm{slab}}$ for slabs of different thicknesses, same area $A$, and same number of water molecules $N_w$ at the surfaces. Then, we calculate $E^{\mathrm{bulk}}_{\mathrm{feldspar}}$ as the slope of a linear fit of the $E_{\mathrm{slab}} - N_w E^{\mathrm{gas}}_{H_2O}$ vs $N_f$ data. With the value of $E^{\mathrm{bulk}}_{\mathrm{feldspar}}$ thus calculated, the surface energy can be obtained via the definition,

$$\gamma = \lim_{N_f \rightarrow \infty} \frac{1}{2A}\left(E_{\mathrm{slab}} - N_w E^{\mathrm{gas}}_{H_2O} - N_f E^{\mathrm{bulk}}_{\mathrm{feldspar}}\right) \tag{16}$$

Note that according to this equation, the surface energy can be lowered either by reducing $E_{\mathrm{slab}}$ or by increasing the

Table 2 Configurations of bulk water, ice $I_h$, and ice $I_c$ used as starting point for training the model. Each row corresponds to a different simulation trajectory. We report the number of configurations extracted from a given trajectory, the phases that were explored, a description of the origin of the simulation trajectory, the time interval between successive frames $\Delta t$, the temperatures or range of temperatures of the simulations $T$, the pressure $P$, and the number of water molecules in the simulation box $N_{H_2O}$.

| # configurations | Phases | Description | $\Delta t$ (ns) | $T$ (K) | $P$ (bar) | $N_{H_2O}$ |
|---|---|---|---|---|---|---|
| 300 | water, ice $I_h$ | Biased simulation [24] | 0.25 | 300-350 | 1 | 96 |
| 300 | water, ice $I_c$ | Biased simulation [24] | 0.25 | 300-350 | 1 | 64 |
| 40 | water | Standard simulation [25] | 1 | 260,270,280,300 | 1 | 288 |
| 200 | LDL, HDL | Standard simulation [26] | 2.5 | 235 | 3200 | 192 |
| 122 | water | Biased simulation [24] | 0.25 | 260-350 | 1 | 64 |

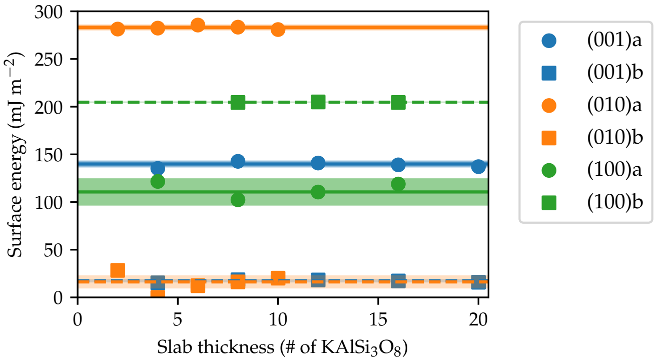


Fig. 2 Zero-temperature surface energy of different fully-hydroxylated terminations of the (100), (010), and (001) surfaces of microcline feldspar vs slab thickness. Fits of a constant function to the data are shown with lines. The width of the semi-transparent regions around each line are one-sigma errors of the fitting procedure.

number of dissociated water molecules $N_w$ at the surface.

The surface energy vs. slab thickness is shown in Fig. 2.

## 8 Formation of ice cluster at the microcline/water interface

The formation of ice at microcline/water interfaces was driven by the following bias potential,

$$V(Q_6^{\text{sph}}(\mathbf{R})) = \frac{k}{2}\left(Q_6^{\text{sph}}(\mathbf{R}) - Q_6^{\text{ctr}}(t)\right)^2 \tag{17}$$

where $k = 10^6$ kJ/mol, $Q_6^{\text{sph}}(\mathbf{R})$ is the Steinhardt parameter localized within a sphere (see definition above), and $Q_6^{\text{ctr}}(t) = Q_6^0 + (Q_6^f - Q_6^0)t/t_{\text{tot}}$ is the center of the harmonic bias which changes linearly with time $t$ from initial value $Q_6^0$ to final value $Q_6^f$ over the total simulation time $t_{\text{tot}} = 10$ ns. $Q_6^0 \approx 0$ and $Q_6^f = 0.4$ are values of $Q_6^{\text{sph}}(\mathbf{R})$ compatible with liquid water and ice, respectively.

## Notes and references


1 P. Giannozzi, S. Baroni, N. Bonini, M. Calandra, R. Car, C. Cavazzoni, D. Ceresoli, G. L. Chiarotti, M. Cococcioni, I. Dabo *et al.*, *J. Phys.: Condens. Matter*, 2009, **21**, 395502.
2 P. Giannozzi, O. Andreussi, T. Brumme, O. Bunau, M. B. Nardelli, M. Calandra, R. Car, C. Cavazzoni, D. Ceresoli, M. Cococcioni *et al.*, *J. Phys.: Condens. Matter*, 2017, **29**, 465901.
3 J. Sun, A. Ruzsinszky and J. P. Perdew, *Phys. Rev. Lett.*, 2015, **115**, 036402.
4 J. Sun, R. C. Remsing, Y. Zhang, Z. Sun, A. Ruzsinszky, H. Peng, Z. Yang, A. Paul, U. Waghmare, X. Wu *et al.*, *Nat. Chem.*, 2016, **8**, 831.
5 M. A. Marques, M. J. Oliveira and T. Burnus, *Comput. Phys. Commun.*, 2012, **183**, 2272–2281.
6 D. Hamann, *Phys. Rev. B*, 2013, **88**, 085117.
7 J. P. Perdew, K. Burke and M. Ernzerhof, *Phys. Rev. Lett.*, 1996, **77**, 3865.
8 L. Bengtsson, *Physical Review B*, 1999, **59**, 12301.
9 L. Zhang, J. Han, H. Wang, R. Car and E. Weinan, *Phys. Rev. Lett.*, 2018, **120**, 143001.
10 H. Wang, L. Zhang, J. Han and E. Weinan, *Comput. Phys. Commun.*, 2018, **228**, 178–184.
11 L. Zhang, J. Han, H. Wang, W. Saidi, R. Car *et al.*, *Adv. Neural Inform. Process. Syst.*, 2018, **31**, 4436–4446.
12 D. Lu, W. Jiang, Y. Chen, L. Zhang, W. Jia, H. Wang and M. Chen, *Journal of chemical theory and computation*, 2022, **18**, 5559–5567.
13 S. Plimpton, *J. Comput. Phys.*, 1995, **117**, 1–19.
14 A. P. Thompson, H. M. Aktulga, R. Berger, D. S. Bolintineanu, W. M. Brown, P. S. Crozier, P. J. in't Veld, A. Kohlmeyer, S. G. Moore, T. D. Nguyen *et al.*, *Comput. Phys. Commun.*, 2022, **271**, 108171.
15 G. Bussi, D. Donadio and M. Parrinello, *J. Chem. Phys.*, 2007, **126**, 014101.
16 G. A. Tribello, M. Bonomi, D. Branduardi, C. Camilloni and G. Bussi, *Comput. Phys. Commun.*, 2014, **185**, 604–613.
17 M. Bonomi, G. Bussi, C. Camilloni, G. A. Tribello,

P. Banáš, A. Barducci, M. Bernetti, P. G. Bolhuis, S. Bottaro, D. Branduardi *et al.*, *Nat. Methods*, 2019, **16**, 670–673.

18 P. Steinhardt, D. Nelson and M. Ronchetti, *Phys. Rev. B*, 1983, **28**, 784–805.

19 J. Van Duijneveldt and D. Frenkel, *J. Chem. Phys.*, 1992, **96**, 4655–4668.

20 P. Rein ten Wolde, M. J. Ruiz-Montero and D. Frenkel, *J. Chem. Phys.*, 1996, **104**, 9932–9947.

21 S. Bailey, *American Mineralogist: Journal of Earth and Planetary Materials*, 1969, **54**, 1540–1545.

22 S. Liu and Y. Zhai, *Periodico di Mineralogia*, 2021, **90**,.

23 H. Kroll and P. H. Ribbe, *American Mineralogist*, 1987, **72**, 491–506.

24 P. M. Piaggi, A. Z. Panagiotopoulos, P. G. Debenedetti and R. Car, *J. Chem. Theory Comput.*, 2021, **17**, 3065–3077.

25 P. M. Piaggi, J. Weis, A. Z. Panagiotopoulos, P. G. Debenedetti and R. Car, *Proc. Natl. Acad. Sci. U.S.A.*, 2022, **119**, e2207294119.

26 T. E. Gartner III, P. M. Piaggi, R. Car, A. Z. Panagiotopoulos and P. G. Debenedetti, *Phys. Rev. Lett.*, 2022, **129**, 255702.

27 L. Zhang, H. Wang, R. Car and W. E, *Phys. Rev. Lett.*, 2021, **126**, 236001.

28 P. Gallo, K. Amann-Winkel, C. A. Angell, M. A. Anisimov, F. Caupin, C. Chakravarty, E. Lascaris, T. Loerting, A. Z. Panagiotopoulos, J. Russo *et al.*, *Chem. Rev.*, 2016, **116**, 7463–7500.

29 L. Zhang, D.-Y. Lin, H. Wang, R. Car and E. Weinan, *Physical Review Materials*, 2019, **3**, 023804.

30 V. Fiorentini and M. Methfessel, *Journal of Physics: Condensed Matter*, 1996, **8**, 6525.
